# Supplementary material for: Pseudo-Euclidean Attract-Repel Embeddings for Undirected Graphs
Source: arXiv:2106.09671 source file (2023-03-23)
Supplement: Supplementary file 1 [file ARDecomp_Supplement.pdf]

## 8 Appendix to “An Attract-Repel Decomposition of Undirected Networks”

### 8.1 Stochastic Block Models

We now look at the relationship of the  $AR$  decomposition to a popular model in the literature: the stochastic block model (SBM) (Holland et al., 1983). These models are used in network analysis in fields as different as looking at human social networks to modeling protein interactions (Airoldi et al., 2006; Abbe, 2017). The SBM works as follows: there are  $d$  blocks. Each node belongs to one block.<sup>6</sup> For blocks  $i, j$  there is a probability  $b_{ij}$  that a node from  $i$  is connected to a node from  $j$ . Let  $B$  be the matrix of node connection probabilities. We assume  $B$  has rank  $d$ . Let  $P_B$  be the implied matrix of probability of connections in a population of  $n$  nodes. Again, ignore the diagonal.

It is known that if  $B$  is positive semi-definite and rank  $k$  then there exists an  $A$  decomposition of rank  $k$  which represents the SBM.

We can generalize this result to the  $AR$  decomposition as well as generalize our example in Figure 1:

**Proposition 6.** *If  $B$  has rank  $d$  then  $P_B$  has the following properties:*

1.  $P_B$  has  $AR$  decomposition of rank  $d$
2. If  $B$  is positive semi-definite then an  $A$  decomposition of  $P_B$  can have rank  $d$
3. If  $B$  has negative eigenvalues then any  $A$  decomposition of  $P_B$  has rank  $> d$ .

*Proof of Theorem 6.* We first prove that  $P_B$  has an  $AR$  decomposition of rank  $k$ . To do this, we will explicitly construct the decomposition. Since  $B$  is symmetric and real it has an  $AR$  decomposition of  $B = XX' - YY'$ . We give each node the embedding corresponding to the embedding of it's block. This is an  $AR$  decomposition of  $P_B$ .

From this the second point follows directly.

The third point follows by contradiction. Suppose that  $P_B$  has an  $A$  decomposition of rank  $d$  (or less). Let this be  $X$ . By construction it must be that all nodes with the same block  $k$  have the same embedding, call it  $x_k$ . But then  $B = XX'$ . But this implies that  $B$  is positive semi-definite, which we know it is not.  $\square$

**Lemma 1.** *The following SBMs will not be positive semi-definite:*

1. **Any SBM with heterophily across blocks:** *There exist some blocks  $i, j$  where nodes in  $i$  are more likely to connect to  $j$  than to  $i$  and nodes in  $j$  are more likely to connect to  $i$  than  $j$ .*
2. **Any SBM with a triangle:** *There are 3 blocks  $i, j, k$  with the properties that*

$$b_{ii}(b_{jj}b_{kk} - b_{jk}^2) - b_{ij}(b_{ij}b_{kk} - b_{jk}b_{ki}) + b_{ik}(b_{ij}b_{jk} - b_{jj}b_{ik}) < 0.$$

*Proof of Lemma 1.* By Sylvester's Criterion for a full rank matrix to be positive semi-definite, any principal minor (submatrix of the same indexed rows and columns) must have non-negative determinant. A  $2 \times 2$  submatrix of  $i, j$  has the determinant

$$b_{ii}b_{jj} - b_{ij}^2$$

where the square is there due to symmetry of  $b_{ij} = b_{ji}$ . If  $b_{ij} > b_{ii}, b_{jj}$  this determinant is negative meaning that  $B$  cannot be positive semi-definite and thus must have negative eigenvalues.

The proof for the second statement in the Lemma is the same, since the equation in the Lemma is in the fact that determinant of a  $3 \times 3$  principal minor.  $\square$

The three-wise case is particularly interesting as we will see later that unclosed triangles play a special role in co-occurrence networks (note the condition in the Lemma is satisfied with a basic triangle where  $i, j$  connect to  $k$  but not to each other  $b_{ii} = b_{jj} = b_{kk} = 1$  and  $b_{ij} = 1, b_{jk} = 1$  but  $b_{ik} = 0$ ).

It is possible to construct higher order interaction conditions that guarantee that  $B$  is not easily  $A$  decomposable but these conditions become harder to interpret.

<sup>6</sup>The extension to a mixed membership model (Airoldi et al., 2008) is straightforward and would not change our main result.

## 498 8.2 Proofs of Main Text Results

499 *Proof of Proposition 1.* Any symmetric matrix  $M$  has a decomposition of the form  $A'A - R'R$ . To  
500 construct this:

- 501 1. Compute the eigendecomposition of  $\hat{P} = Q'DQ$ . Any symmetric matrix has such a decom-  
502 position with real eigenvalues.
- 503 2. Let  $D^-$  be the negative eigenvalues and  $D^+$  be the positive ones. Let  $Q^-$  correspond  
504 to the eigenvectors with negative eigenvalues and  $Q^+$  be the eigenvectors with positive  
505 eigenvalues.
- 506 3. Let  $A = Q^+\sqrt{D^+}$  and let  $R = Q^-\sqrt{-D^-}$

507 Since given any diagonal matrix  $D$  the matrix  $M + D$  is still symmetric, the decomposition continues  
508 to exist. The family of AR decompositions is thus equivalent to any choice of diagonal for  $M$ .  $\square$

*Proof of Proposition 2.* By Lemma 6 of Mazumder et al. (2010) we know that for a matrix  $X$  we can  
write

$$\|X\|_* = \min_{UV=X} \frac{1}{2}(\|U\|_F^2 + \|V\|_F^2).$$

509 With the minimum being attained at the factor decomposition  $X = UV$ .

510 By construction of our matrix  $\tilde{M}$  it has the factor decomposition  $U = [A, R]$  and  $V = [A, -R]$   
511 where  $[\cdot]$  denotes column-wise concatenation.

Substituting the definition of the factors gets

$$\|\tilde{M}\|_* = \frac{1}{2}(2 \sum_{ij} a_{ij}^2 + 2 \sum_{ij} r_{ij}^2)$$

which simplifies to

$$\|\tilde{M}\|_* = \|A\|_F^2 + \|R\|_F^2.$$

512 Recall the construction of  $\tilde{M}$  is by finding the smallest  $A, R$  in terms of  $\|A\|_F^2 + \|R\|_F^2$  to fit all  
513 the off diagonal elements. Thus, these  $A, R$  also solve the constrained nuclear norm minimization  
514 problem.  $\square$

515 *Proof of Proposition 3.* We know that any symmetric matrix  $C$  that is positive semi-definite has a  
516 decomposition of the form  $C = A'A$ . Thus it is sufficient to show there exists a choice of diagonal  
517  $D$  such that  $M - D$  is positive semi-definite. Let  $\Delta$  be the eigenvalues of  $M$ . If all  $\Delta$  are weakly  
518 positive we are done since then  $M$  is positive semi-definite. Let  $\delta$  be the largest negative eigenvalue  
519 otherwise. Construct the diagonal  $D_\delta$  as the constant  $-\delta$ .

520 Given a matrix  $M$  the eigenvalues of  $M + D$  are simply the eigenvalues of  $M$  shifted up by  $D$ .  
521 Therefore, by construction  $M - D_\delta$  has non-negative eigenvalues. But then it is positive semi-definite.  
522 Let  $A_\delta$  be the decomposition of  $M - D_\delta$ . Then  $M = D_\delta + A'_\delta A_\delta$  as required.  $\square$

523 *Proof of Proposition 4.* In essence, we want to determine the rank, that is, determine the dimension  
524 of the nullspace of a matrix

$$M = \begin{pmatrix} A & R \\ R & B \end{pmatrix}$$

525 where  $A$  is an  $n \times n$  diagonal matrix with coefficients  $a_1 \dots a_n > 0$ ,  $B$  is an  $n \times n$  diagonal matrix  
526 with coefficients  $b_1 \dots b_n > 0$ , and  $R$  is an  $n \times n$  matrix of all 1. Let's solve!

$$M \times \begin{pmatrix} \mathbf{u} \\ \mathbf{v} \end{pmatrix} = 0 \iff \forall i \begin{cases} a_i u_i + \sum_j v_j = 0 \\ b_i v_i + \sum_j u_j = 0 \end{cases}$$

527 Since  $a_i > 0$  and  $b_i > 0$ , this implies

$$\forall i \quad u_i = -\frac{1}{a_i} \sum_j v_j \quad v_i = -\frac{1}{b_i} \sum_j u_j \quad (3)$$

528 If we were free to set  $\sum_j v_j$  and  $\sum_j u_j$  as we please, the two equations (3) would describe a 2-  
 529 dimensional space. Therefore the nullspace of  $M$  has dimension at most 2. However we can also use  
 530 the first of these equations to write

$$\sum_i u_i = -\sum_i \frac{1}{a_i} \sum_j v_j \quad (4)$$

531 Therefore our nullspace has dimension at most 1. But we can continue and use the second equations  
 532 from (3) to replace  $v_j$  above:

$$\sum_i u_i = -\left(\sum_i \frac{1}{a_i}\right) \left(\sum_j v_j\right) = \left(\sum_i \frac{1}{a_i}\right) \left(\sum_j \frac{1}{b_j}\right) \sum_k u_k$$

533 Therefore, if  $r = \left(\sum_i \frac{1}{a_i}\right) \left(\sum_j \frac{1}{b_j}\right) \neq 1$ , then we must have  $\sum_i u_i = \sum_j v_j = 0$  which means that  
 534  $u_i = v_j = 0$ : the matrix is nonsingular. On the other hand, if  $r = 1$ , then I can choose  $\sum_j v_j$  equal  
 535 to any non zero value, deduce  $\sum_j u_i$  using (4), compute  $u_i$  and  $v_i$  using (3), and verify that we have  
 536 described a one-dimensional nullspace.

537 In conclusion: if  $r = \left(\sum_i \frac{1}{a_i}\right) \left(\sum_j \frac{1}{b_j}\right) \neq 1$ , the matrix has full rank. If  $r = 1$  the matrix has rank  
 538  $2n - 1$ . This is the case, for instance, when  $a_i = b_j = n$ .  $\square$

539 *Proof of Proposition 5.* Let  $D$  be the data matrix for all legal combinations of the sandwich problem.  
 540 Consider the matrix  $C = D'D$  which is the  $2M \times 2M$  co-occurrence matrix of all items that are  
 541 purchased. We know that  $\text{rank}(C) \leq \text{rank}(D)$ .

542 It is easy to check that if  $i$  be a meat and  $j$  be a bread (or vice versa) then  $c_{ij} = 1$ . If  $i, j$  are  
 543 the same item type, then  $c_{ij} = 0$ . For any  $c_{ii} = M$ . This is precisely the matrix described in the  
 544 proof of Proposition 4. This matrix has rank  $2M - 1$ . Therefore the matrix  $D$  also has rank at least  
 545  $2M - 1$ .  $\square$
